# Supplementary material for: EgoXperience: Learning World-Grounded Egocentric Representations from Human Experience
Source: arXiv:2610.26625 source file (2026-10-19)
Supplement: Supplementary file 1 [file additional_results.tex]

\section{Additional Results}
\label{appendix:additional_results}

Use this appendix for complete per-dataset tables, per-regime breakdowns, failure cases, and extra qualitative examples.
Keep the main paper focused; put exhaustive tables here.

\input{tabs/appendix/per_dataset_results_template}
