# Supplementary material for: EgoXperience: Learning World-Grounded Egocentric Representations from Human Experience
Source: arXiv:2610.26625 source file (2026-10-19)
Supplement: Supplementary file 2 [file implementation_details.tex]

\section{Implementation Details}
\label{appendix:implementation_details}

Use this appendix section to document details that affect reproducibility but would interrupt the main narrative.
Typical Ropedia papers should include the exact data preprocessing version, model checkpoints, training schedule, evaluation hardware, inference resolution, and any filtering thresholds.

\subsection{Data Format}

Describe the released per-scene directory layout and metadata schema.
For dataset or benchmark papers, list required files such as RGB frames, depth maps, camera intrinsics, camera-to-world poses, masks, and split files.

\subsection{Training and Inference}

Report optimizer, batch size, learning rate schedule, input resolution, augmentation, number of iterations or epochs, and compute budget.
If the paper releases model checkpoints, state which checkpoint is used for every reported table.

\subsection{Evaluation}

State the exact evaluation command or configuration file used for the main tables.
For benchmark papers, include how invalid predictions, missing outputs, OOM, and timeout cases are handled.
