# Supplementary material for: EgoXperience: Learning World-Grounded Egocentric Representations from Human Experience
Source: arXiv:2610.26625 source file (2026-10-19)
Supplement: Supplementary file 3 [file limitations.tex]

\section{Limitations and Broader Impact}
\label{appendix:limitations}

Use this section to make the boundary of the Ropedia release clear.
Discuss known data coverage gaps, annotation noise, hardware constraints, benchmark blind spots, and deployment considerations.

\textbf{Limitations.}
List the most important constraints of the dataset, method, or benchmark.
Be specific about domains where performance has not been validated.

\textbf{Broader impact.}
For egocentric or embodied datasets, describe privacy, consent, data governance, and responsible release considerations.
For model releases, describe potential misuse, failure modes, and recommended evaluation before deployment.
