# Supplementary material for: EgoXperience: Learning World-Grounded Egocentric Representations from Human Experience
Source: arXiv:2610.26625 source file (2026-10-19)
Supplement: Supplementary file 4 [file ropedia_curation.tex]

\section{Ropedia Data Curation Pipeline}
\label{appendix:ropedia_curation}

This appendix section is adapted from the current SpatialBench Xperience appendix.
Use it to give the operational details that are too dense for the main paper.

\subsection{Xperience-Style Pipeline}

Xperience~\citep{xperience_10m} consists of egocentric sequences captured with a head-mounted device during human activity.
The current pipeline samples a subset of the original data, estimates camera poses using a SLAM system built upon ViPE~\citep{huang2025vipe}, and estimates metric depth maps plus confidence maps from rectified stereo image pairs using FoundationStereo~\citep{wen2025foundationstereo}.

\subsection{Recommended Reporting Checklist}

\begin{itemize}
  \item Raw data source and license.
  \item Sensor setup, frame rate, resolution, and synchronization assumptions.
  \item Pose estimation or reconstruction system.
  \item Depth, mask, segmentation, or tracking annotation source.
  \item Filtering thresholds and sequence rejection criteria.
  \item Released file format and per-scene metadata schema.
\end{itemize}
