# Supplementary material for: EgoXperience: Learning World-Grounded Egocentric Representations from Human Experience
Source: arXiv:2610.26625 source file (2026-10-19)
Supplement: Supplementary file 5 [file per_dataset_results_template.tex]

\begin{table}[t]
\centering
\caption{\textbf{Appendix Per-Dataset Results Template.}
Use this table for expanded metrics that are too detailed for the main paper.
Use \texttt{rankfirst}, \texttt{ranksecond}, and \texttt{rankthird} for the Ropedia green ranking palette defined in \texttt{macro.tex}.
}
\label{tab:appendix_per_dataset_results_template}
\resizebox{\textwidth}{!}{%
\renewcommand{\arraystretch}{1.12}
\setlength{\tabcolsep}{5pt}
\begin{tabular}{l >{\columncolor{subcol}}c c >{\columncolor{subcol}}c c >{\columncolor{subcol}}c c}
\toprule
\multirow{2.5}{*}{\textbf{Method}}
& \multicolumn{2}{c}{\textbf{Depth}}
& \multicolumn{2}{c}{\textbf{Pose}}
& \multicolumn{2}{c}{\textbf{Trajectory}} \\
\cmidrule(lr){2-3}\cmidrule(lr){4-5}\cmidrule(lr){6-7}
& AbsRel$\downarrow$ & RMSE$\downarrow$ & AUC@30$\uparrow$ & RRA@15$\uparrow$ & ATE$\downarrow$ & RPE$_t\downarrow$ \\
\midrule
Baseline A & 0.000 & 0.000 & 0.000 & 0.000 & 0.000 & 0.000 \\
Baseline B & 0.000 & 0.000 & 0.000 & 0.000 & 0.000 & 0.000 \\
\ours (Ours) & \cellcolor{rankfirst}\textbf{0.000} & \cellcolor{rankfirst}\textbf{0.000} & \cellcolor{rankfirst}\textbf{0.000} & \cellcolor{rankfirst}\textbf{0.000} & \cellcolor{rankfirst}\textbf{0.000} & \cellcolor{rankfirst}\textbf{0.000} \\
\bottomrule
\end{tabular}%
}
\end{table}
